# Supplementary material for: SAIL: Sample-Centric In-Context Learning for Document Information Extraction
Source: arXiv:2412.17092 source file (2024-12-22)
Supplement: Supplementary file 1 [file 0.overview.tex]

\section{Overview}

This \supp is structured as follows. 
More implementation details are described in \ref{supp:sec:implementation}, followed by additional ablation experiments in \ref{supp:sec:ablation}. 
Significance analysis and more visual examples are presented in \ref{supp:sec:result}.
